# Supplementary material for: Dissecting Distribution Inference
Source: arXiv:2212.07591 source file (2024-04-05)
Supplement: Supplementary file 1 [file additional_figures.tex]

\subsection{Additional Figures} \label{app:additional_figs}
